# Supplementary material for: The Central Spanning Tree Problem
Source: arXiv:2404.06447 source file (2024-04-09)
Supplement: Supplementary file 1 [file 2organize.tex]

\section{Introduction references to appendix}
\begin{itemize}
    \item Prove why $m_e*(1-m_e)$ is equal to the centrality of a edge in a tree. Done in footnote
    \item Prove equivalence \MRCT classical formulation and flow based one (Mentioned already in introduction)
    \item Limit cases of the \CST objective function when $\alpha\to\pm\infty$
    \item CST as a MCCNF. Explain first how $m_e$ can be seen as a flow. This is common foundation to build from for the BOT and MCCNF relation.
\end{itemize}

\section{Stabiliity toy data references to appendix}
\begin{itemize}
    \item Evolution of tree with respect to alpha for sample and noisy sample
\end{itemize}

\section{Correspondence BCST and CST references to appendix}
\begin{itemize}
    \item 4 degree BP
    \item number CST topogies derived from BCST and viceversa
    \item counterexample optimum BCST is not derived from optimum CST and viceversa
\end{itemize}

\section{Optimization CST references to appendix}
\subsection{Geometry Optimization BCST references to appendix}
\begin{itemize}
    \item Differences and similarities with the BOT problem
    \item Show independence of weight factors of the geometry optimization step.
\end{itemize}

\subsection{Heuristic references to appendix}
\begin{itemize}
    \item Explication of the effect of frequency sampling inside edges-> \figurename{} \ref{fig:mSTreg_freqsampling} shows different sampling frequencies per edge for the example of \figurename{} \ref{sfig2:mSTreg_scheme}.\TODO{move to appendix}%TODO

    \item Reference to heuristic pseudocode.
    \item Explain heuristics to merge BPs
\end{itemize}

\subsection{Benchmark references to appendix}
\begin{itemize}
    \item Brute-force plots for different alpha values
\end{itemize}

\section{Implemetation Details}
\begin{itemize}
    \item Explain parameters experiments
\end{itemize}

\section{geometry optimization algorithm}
%%%%%%%%%%%%%%%%%%%%%%%%%%%%%%%%
Indeed, we can calculate the gradient of the objective function \eqref{eq:CST_nonnorm} and equate it to zero. We obtain the following linear system
\begin{equation}
x_i=\frac{\displaystyle\sum_{j: i,j\in E_T}\frac{\big(m_{ij}(1-m_{ij})\big)^{\alpha}x_j}{|x_i-x_j|}}{\displaystyle\sum_{j: i,j\in E_T}\frac{\big(m_{ij}(1-m_{ij})\big)^{\alpha}}{|x_i-x_j|}}
\end{equation}
This linear system can be solved via iteratively reweighted least squares (IRLS) efficiently. 
%%%%%%%%%%%%%%%%%%%%%%%%%%%%%%%%%%%%%%%%%%%%%%%%%%%%%%%

\section{Number topologies derived from \BCST topology}
We can use the \BCST topology given by our heuristic to infer a solution for the \CST problem without branching points. In this case we need to collapse BPs. As it was the case for the computation of a full tree topology, the inverse process is ambiguous, i.e. we can obtain different spanning trees connecting the terminals from a full tree topologies. The number of topologies that one can obtain from a full tree topology $T$ is given by \TODO{Move formula and proof to appendix and just mention that it is of order O($3^N$)}%TODO
\begin{equation}
	\label{eq:number_topos_derived_from_fulltopo}
	3^{N-2-K(T)}\sum_{i=1}^{K(T)+N+1}\left(3^{K(T)-i}|\mathcal{N}(x_{N+1+K+i})\cap X_t|\prod_{j=N+1}^{i+K(T)-1}\left(3-|\mathcal{N}(x_j)\cap X_t|\right)\right)
\end{equation}
where $X_t$ represent the set of terminals, $\mathcal{N}(x_i)$ indicates the set of neighbors of node $x_i$ and $K(T)$ is the number of BPs which are neighbor of a terminal node, i.e. the cardinality of the set $\{x_i \ : \ |\mathcal{N}(x_j)\cap X_t|>0\}=\{N+1,N+2,\dots,N+1+K(T)\}$.\footnote{W.L.O.G we assume that the BPs numbered from $N+1$ to $K+N+1$ are the BPs which are neighbors of at least one terminal node.} The logic behind \eqref{eq:number_topos_derived_from_fulltopo} is the following: each BP has 3 neighbors, thus it can be collapsed to any of their neighbors. Naively we could say that there are $3^{N-2}$ topologies since each BP has 3 options to collapse and there $N-2$ BPs. That is not the case, since it is not a valid topology where all BPs choose to collapse to a neighbor which is also a BP, since if we do these collapses sequentially the last BP would be the result of collapsing all the BPs and therefore it should collapse with itself. To be valid, we need that at least one of the BPs collapses with a terminal node. The sum takes this into account. In concrete the sum iterates over the BPs that are neighbor of a terminal and considers the cases where the BP $i$ collapses with a terminal and the rest of BPs do a free choice. In the next iteration of the sum, we won't allow the BP $i$ to collapse to a terminal neighbor but to a BP neighbors in order to avoid repeated topologies. This is why we need the product inside the sum, which keeps track of the BPs, whose terminal neighbor collapse have already been explored.

\subsection{\CST topo to \BCST}
 For each terminal, $v$, with degree $d_v\geq 2$, we need to create $d_v-1$ BPs. There are $(2d_v-5)!!$ ways of connecting these BPs to the neighbors of $v$.
 
\section{\mSTreg }
 
 \IncMargin{1.6em}
 \begin{algorithm}
 	
 	\caption{CST: mST regularization heuristic}\label{alg:CST_mSTreg}
 	
 	\DontPrintSemicolon
 	\Indm  
 	\KwInput{$X$, num\_reguralizations, sampling\_frequency}
 	\KwOutput{Tree}
 	\Indp  
 	
 	\tcc{Define initial topology as mST}
 	$mST_{init}=$minimum\_spanning\_tree(X)\\\BlankLine
 	\tcc{transform topology to full topology}
 	$T_{CST}=$transform2fulltopo($mST_{init}$)\\\BlankLine 
 	\tcc{compute branching point positions}
 	$T_{CST},BP$=compute\_BP($T_{init}$)\\\BlankLine 
 	bestcost=$\infty$\\
 	\While{$it<$num\_reguralizations}{
 		\If{sampling\_frequency$>$2}
 		{
 			\tcc{sample extra points from edges}
 			Y=sample\_from\_edge($T_{CST}$,$X\cup BP$,sampling\_frequency)\\
 			$BP=BP\cup Y$
 		}
 		$mST_{X\cup BP}$=minimum\_spanning\_tree($X\cup BP$)\\\BlankLine 
 		\tcc{remove BP from $mST_{X\cup BP}$ and ensure full topology}
 		$T_{CST}=$transform2fulltopo($mST_{X\cup BP}$)\\\BlankLine 
 		\tcc{compute branching point positions}
 		$T_{CST},BP$=compute\_BP($T_{reg}$)\\
 		\tcc{Store topology if cost is improved}
 		\If{cost($T_{CST})<$bestcost}
 		{
 			bestcost=cost($T_{CST})$\\
 			$T_{CST best}=T_{CST}$
 		}	
 		
 	}
 	
 \end{algorithm}
 \DecMargin{1.6em}
 \subsection{Effect higher frequency sampling in \mSTreg}
\input{Figures/mSTREG_freqsampling.tex}
