# Supplementary material for: The Central Spanning Tree Problem
Source: arXiv:2404.06447 source file (2024-04-09)
Supplement: Supplementary file 2 [file limit_cases_CST_positive_limit.tex]

\subsection{Topology Analysis in the Limit Case of $\alpha\to\infty$}\label{sec:app_limitCST_positive}
In this case, the tree topology will tend to a star graph centered at the medoid. The medoid is defined as node that minimizes the total distance to all other nodes. When $\alpha$ is high, the \CST  aims to minimize the centrality of the edges, since the edge costs become relatively insignificant in comparison. Among all edges of a tree, the ones adjacent to a leave have the least centrality. Thus, any star graph is a tree that minimizes simultaneously the edge centrality of all its edges, with each of them having centrality equal to $(N-1)/N$ (see \thref{lem:tree_opt_alpha_inf}). In such case, we can factor out the edge centrality of the cost function in \eqref{eq:CST} and the problem reduces to find the star graph with minimum cost. As a result, when $\alpha$ tends to positive infinity, the optimal solution of the problem \CST will be a star graph centered at the node that minimizes the total distance to all other nodes, that is, centered at the medoid. In the case of the \BCST,  where Steiner Points can be added, the star graph will be centered at the geometric median, as the Steiner Points will adjust to the location that minimizes the distance to all nodes.

The next Lemma formalizes why star graphs have lower cost than non-star graphs for $\alpha$ high enough in the \CST problem.

\begin{lemma}\thlabel{lem:tree_opt_alpha_inf}
As $\alpha$ approaches infinity ($\alpha\to\infty$), for any non-star-shaped tree $T$, there exists a star graph $T_{\star}$ with a lower \CST cost.
\end{lemma}
\begin{proof}
    We will demonstrate that it is always possible to increase the degree of a specific node in such a way that the \CST cost of $T$ decreases. This process can be repeated until a single node with a degree of $N-1$ is reached, resulting in the formation of a star graph.
    
    Let $e=(u,v)$ be the most central edge of $T$. Let us assume w.l.o.g.~ that the number of nodes at $u$'s side of edge $e$ has more nodes than the side of $v$. Let $k\neq u\in \mathcal{N}_v$. We will show that the topology $T'$ which connects $k$ to $u$ instead of $v$ has a lower \CST cost. The only edge centralities affected by this change are those associated with edges $(u,v)$, $(u,k)$, and $(k,v)$. To compare the costs of the topologies, it suffices to focus on these specific edges.

        First, let's determine the values of the centralities for the edges in both trees:
    \begin{itemize}
        \item  Normalized centrality of edge $(u,v)$ in $T$:
            $$m^T_{uv}(1-m^T_{uv})$$
        \item  Normalized centrality of edge $(u,v)$ in $T'$: 
            $$m^{T'}_{uv}(1-m^{T'}_{uv})=\left(m^{T}_{uv}+m^{T}_{kv}\right)\left(1-m^{T}_{uv}-m^{T}_{kv}\right)$$
            The equality is a result of the fact that once $k$ becomes a neighbor of $u$, all nodes that were on the same side as $k$ will now be on the same side as $u$.
        \item Normalized centrality of edge $(k,v)$ in $T$ and centrality of edge $(k,u)$ in $T'$: 
            $$m^T_{kv}(1-m^T_{kv})=m^{T'}_{ku}(1-m^{T'}_{ku})$$
            Both $u$ and $v$ lie in the same side of the edges, hence the equality of their normalized centralities.
    \end{itemize}
    Note that $m^{T'}_{uv}(1-m^{T'}_{uv})<m^{T}_{uv}(1-m^{T}_{uv})$, since we are adding more nodes to the side of $u$ which already had a greater number of nodes than the side of $v$. Additionally, since the side of $u$ already had more nodes than the side of $v$, we have $m^{T}_{uv}>0.5$. The difference between the costs of the topologies is
    \footnotesize\begin{equation}
        \begin{aligned}\label{eq:tree_opt_alpha_inf}
        \operatorname{CST}(T)-\operatorname{CST}(T')=&c_{uv}\left(m^T_{uv}\big(1-m^T_{uv}\big)\right)^{\alpha}+c_{kv}\left(m^T_{kv}\big(1-m^T_{kv}\big)\right)^{\alpha}\\
           &-c_{uv}\left(\left(m^{T}_{uv}+m^{T}_{kv}\right)\left(1-m^{T}_{uv}
           -m^{T}_{kv}\right)\right)^{\alpha}
           -c_{ku}\left(m^T_{kv}\big(1-m^T_{kv}\big)\right)^{\alpha}\\
           =&c_{uv}\Bigg(\left(m^T_{uv}\big(1-m^T_{uv}\big)\right)^{\alpha}-\left(\left(m^{T}_{uv}+m^{T}_{kv}\right)\left(1-m^{T}_{uv}-m^{T}_{kv}\right)\right)^{\alpha}\Bigg)\\
           &+(c_{kv}-c_{ku})\left(m^T_{kv}\big(1-m^T_{kv}\big)\right)^{\alpha}\\
           %%%%%%%%%%%%%%%%%%%%%%%%%%%%%%%%%%%%%%%%%%%%%%%%%%%%%
           =&\frac{c_{uv}}{m^T_{kv}}\Bigg(\frac{\left(m^T_{uv}\big(1-m^T_{uv}\big)\right)^{\alpha}-\left(\left(m^{T}_{uv}+m^{T}_{kv}\right)\left(1-m^{T}_{uv}-m^{T}_{kv}\right)\right)^{\alpha}}{m^T_{kv}}\Bigg)
           \\&+(c_{kv}-c_{ku})\left(m^T_{kv}\big(1-m^T_{kv}\big)\right)^{\alpha}\\
           %%%%%%%%%%%%%%%%%%%%%%%%%%%%%%%%%%%%%%%%%%%%%%%%
           \geq&\frac{c_{uv}}{m^T_{kv}}\frac{dF}{dx}\left[m^T_{uv}\right]+ (c_{kv}-c_{ku})\left(m^T_{kv}\big(1-m^T_{kv}\big)\right)^{\alpha}
        \end{aligned}
    \end{equation}
    %%%%The inequality is right because funcion G(y)=(((x+y)(1-x-y)^)alpha)/y is decreasing with respect to y if 
    %x>0.5 and x+y<1. Thus x/y-G(y) will be increasing.
    \normalsize
    where $F(x)=\left(x(1-x)\right)^\alpha$ and $\frac{dF}{dx}[\hat{x}]$ denotes its derivative evaluated at $\hat{x}$. In the inequality, we used the fact that the function $(F(x)-F(x+h))/h$ is decreasing with respect to $h$ when $x>0.5$ and $x+h<1$. As $h$ approaches 0, we recover the derivative of $F$.
    
    By utilizing the fact that $\left(m^T_{kv}\big(1-m^T_{kv}\big)\right)\leq\left(m^T_{uv}\big(1-m^T_{uv}\big)\right)$ which follows from $(u,v)$ being the most central edge of $T$, we can proceed with the following calculations:
    \begin{align*}
        \frac{F(m^T_{kv})}{\frac{dF}{dx}[m^T_{uv}]}&=\frac{(c_{kv}-c_{ku})(m^T_{kv}(1-m^T_{kv}))^{\alpha}}{\alpha(m^T_{uv}(1-m^T_{uv}))^{\alpha-1}(2m^T_{uv}-1)}\\
        &\leq\frac{\displaystyle\sum_{\substack{k\in\mathcal{N}_v \\k\neq u}}(c_{kv}-c_{ku})(m^T_{uv}(1-m^T_{uv}))^{\alpha}}{\alpha(m^T_{uv}(1-m^T_{uv}))^{\alpha-1}(2m^T_{uv}-1)}\\
        &=\frac{(c_{kv}-c_{ku})m^T_{uv}(1-m^T_{uv})}{\alpha(2m^T_{uv}-1)}\xrightarrow{\alpha\to\infty}0
    \end{align*}
    Hence, for $\alpha$ high enough the first term of the last expression in \eqref{eq:tree_opt_alpha_inf} will dominate the second term resulting in a positive difference between $\CST(T)$ and $\CST(T')$. By repeating this process, we will eventually arrive at a star graph with a lower cost than the original tree $T$.
\end{proof}

Next Lemma shows that in the \BCST case, the Steiner points tend to collapse with each other as $\alpha$ approaches infinity, forming a star-shaped graph.

\begin{lemma}\thlabel{lem:tree_opt_alpha_inf_BCST}
For any given topology $T$, as $\alpha$ approaches infinity ($\alpha\to\infty$), there exists a geometric arrangement in which all Steiner points are collapsed into a single node that has a lower \BCST cost than any other arrangement where not all Steiner points are collapsed.
\end{lemma}
\begin{proof}
    
    Consider $T$ as a topology in which not all Steiner points have been collapsed into a single point. Let $b$ represent the Steiner point that is adjacent to the edge with the highest centrality among all edges.  We will demonstrate that collapsing all Steiner points with the Steiner point $b$ reduces the \BCST cost. 
    
    We denote the centrality of the edge connecting nodes $u$ and $v$ as $\zeta_{uv} = m_{uv}(1 - m_{uv})$, and we represent the distance between nodes $u$ and $v$ as $d_{uv}$. Let $\zeta_* \coloneqq \max \zeta_{uv}$. It is important to note that although $T$ does not collapse all Steiner points into one, the Steiner point $b$ may have already been collapsed with other Steiner points. In such cases, we consider the collapsed nodes as single one represented by the node $b$. Thus, $b$ may have degree higher than three and the distance from $b$ to all its neighbors is strictly positive, i.e. $d_{bu}>0$ for all nodes, $u$, neighboring $b$.  We denote by $T'$ the solution obtained by collapsing all Steiner points with node $b$, while preserving the topology. Note that in $T'$, only the distances have been updated, while the edge centralities remain the same as in $T$. Let $d_{uv}'$ represent the distances of $T'$. Notice that $d'_{ub} = 0$ for all Steiner points $u$ neighboring $b$, as all Steiner points have been collapsed to $b$. Now we are able to show that the cost of $T'$ is lower than the one of $T$ as $\alpha$ approaches infinity.
    \begin{equation}
        \begin{aligned}\label{eq:tree_opt_alpha_inf_BCST}
        \operatorname{BCST}(T)-\operatorname{BCST}(T')&=\sum_{(u,v)\in E_T}d_{uv}\zeta_{uv}^\alpha-\sum_{(u,v)\in E_T}d'_{uv}\zeta_{uv}^\alpha=\sum_{(u,v)\in E_T}(d_{uv}-d_{uv}')\zeta_{uv}^\alpha\\
        &=\zeta_*^\alpha\underbrace{\left(\sum_{(u,v)\in E_T\backslash E_{\zeta_*}}(d_{uv}-d_{uv}')\Big(\underbrace{\frac{\zeta_{uv}}{\zeta_*}}_{<1}\Big)^\alpha+\sum_{(u,v)\in E_{\zeta_*}}(d_{uv}-\underbrace{d_{uv}'}_{=0})\right)}_{\xrightarrow{\alpha\to\infty}\sum_{(u,v)\in E_{\zeta_*}}d_{uv}>0}
        \end{aligned}
    \end{equation}
    where $E_{\zeta_*}\coloneqq\{(u,v)\in E_T \ : \ \zeta_{uv}=\zeta_* \}$. Note that we have utilized the fact that all edges in $E_{\zeta_*}$ are connected to $b$, implying that $d_{uv}'=0$ for all $(u,v) \in E_{\zeta_*}$. Consequently, based on Equation \eqref{eq:tree_opt_alpha_inf_BCST}, it follows that for a sufficiently high value of $\alpha$, the cost of $T'$ is lower than the one of $T$. This demonstrates the existence of a more optimal star-shaped arrangement of the Steiner points as $\alpha$ approaches infinity.
\end{proof}

\begin{corollary}
As $\alpha$ approaches infinity ($\alpha\to\infty$), the \CST optimal solution is the star-shaped tree centered at the medoid of the terminals, that is, centered at the terminal which minimizes the sum of distances to all nodes. For the \BCST case, the tree is centered at the geometric median of all terminals.
\end{corollary}
\begin{proof}
    As a  consequence of \thref{lem:tree_opt_alpha_inf}, the optimal solution must be a star graph. In a star graph all edges have the same centrality, which is equal to $N-1/N$, where $N$ is the number of terminals.
    Let $u$ denote the center node of a star graph, then its \CST objective is equal to
    \[\sum_{v\neq u }\frac{N-1}{N}c_{uv}=\frac{N-1}{N}\sum_{v\neq u }c_{uv}.\]
    Thus the optimum star-graph is the one whose center minimizes $\sum_{v\neq u }c_{uv}$, i.e. the star-graph centered at the medoid. The analogous argument can be applied for the \BCST case.
    
\end{proof}
