# Supplementary material for: The Central Spanning Tree Problem
Source: arXiv:2404.06447 source file (2024-04-09)
Supplement: Supplementary file 3 [file num_topos_ERROR_derivable_CST_BCST.tex]

\subsection{Number of BCST topologies derivable from a CST topology.}
In this section, we explicitly determine the number of topologies of the \BCST problem that can be derived from a single \CST topology. 

To derive a full tree topology $T_{\BCST}$ from a \CST topology $T_{\CST}$ with $N$ terminals, we need to add $N-2$ \SPs. In particular, for each terminal node, $v$, with degree $d_v\geq 2$, we need to spawn $d_v-1$ \SPs. Since for $k$ terminal nodes, there exist a total $(2k-5)!!$ of full tree topologies \cite{schroder_vier_1870}, there are $(2(d_v+1)-5)!!=(2d_v-3)!!$ ways to connect the added \SPs to the neighbors of $v$ and $v$ itself. Thus the total number of full tree topologies is equal to the number of possible combinations of subtopologies engendered per terminal neighborhood for terminals with degree higher than 2. Formally, this number is equal
\begin{equation}
    \prod_{v\ :\ d_v\geq 2} (2d_v-3)!!.
\end{equation}
Note that, on the one hand, if all nodes have degree lower or equal than $2$, i.e. the tree is a path, then a single full tree topology can be derived. On the other hand, if the original $T_{\CST}$ is a star graph, then there is a single graph with degree higher than $2$, which is equal to $N-1$. Thus, the total number of topologies derived from it is equal to $(2N-5)!!$. This is the total number of possible full tree topologies, hence a star graph can generate any full tree topology. In general, the higher the degree of the nodes in $T_{\CST}$, the higher the number of derivable full tree topologies.

\subsection{Number of CST topologies derivable from a BCST topology.}\label{subsec:app_numtopos_CST}
In this section, we explicitly determine the number of topologies of the \CST problem that can be derived from a single \BCST topology. 

In this case, we need to collapse each \SP to a terminal. Let $V=\{v_1,\dots,v_N\}$ denote the set of terminals, and $B=\{v_{N+1}\dots,v_{2N-2}\}$ the set of \SPs. Moreover, w.l.o.g we assume that the \SPs numbered from $N+1$ to $K+N+1$ are the ones neighboring at least one terminal node. Here, $K$ represents the total number of such \SPs.
The number of topologies that can be obtained from a full tree topology $T_{\BCST}$ is given by 
\begin{equation}
	\label{eq:number_topos_derived_from_fulltopo}
	3^{N-2-K}\sum_{i=1}^{K}\left(|\mathcal{N}(v_{N+i})\cap V| 3^{K-i}\prod_{j=N+1}^{N+1+i}\left(3-|\mathcal{N}(v_j)\cap V|\right)\right)
\end{equation}
The logic behind equation \eqref{eq:number_topos_derived_from_fulltopo} is as follows: each \SP can be collapsed to any of their neighbors. Naively, we might think there are $3^{N-2}$ topologies since each \SP has 3 neighbors to collapse with and there are $N-2$ \SPs. However, this is not the case because some combinations result in non-valid topologies. For example, when all SPs collapse with a neighbor that is also an SP, none of the SPs have been collapsed with a terminal. To avoid non-valid topologies, we enforce that at least one of the \SPs having a terminal as neighbor, say $v_{N+i}$, must be collapsed with a neighboring terminal. \SP $v_{N+i}$ can choose to collapse with as many neighboring terminals as it has, i.e. with $|\mathcal{N}(v_{N+i})\cap V|$ terminal nodes. This term is the first that appears inside the sum. The sum iterates over the \SPs that are neighbors of a terminal. 

Still, the collapse process may be redundant. To avoid redundancy, after forcing an \SP to collapse with a neighboring terminal, in the subsequent iterations, we force it to collapse with the neighboring SPs. This term is represented by the term $\prod_{j=N+1}^{N+1+i}\left(3-|\mathcal{N}(v_j)\cap V|\right)$. Consequently, no topology is repeated.

In summary, each term of \eqref{eq:number_topos_derived_from_fulltopo} has the following purpose
\begin{itemize}
    \item $3^{N-2-K}$: Counts the number of collapse combinations that have all \SPs not neighboring a terminal. Each of them has 3 possibilities and there are $N-2-K$ \SPs not neighboring a terminal.
    
    \item $\displaystyle \sum_{i=1}^{K}$: Iterates over the \SPs that neighbor a terminal.
    
    \item $|\mathcal{N}(v_{N+i})\cap V|$: For \SP $v_{N+i}$, which is forced to collapse with a neighboring terminal, it counts the number of terminal choices it has, i.e. how many of its neighbors are terminals.
    
    \item $3^{K-i}$: Counts the number of combinations of collapse choices for all \SPs with a neighboring terminal that have not been yet forced to collapse with a terminal. Each of them has the free choice to merge with any of its three neighbors.
    
    \item $\prod_{j=N+1}^{N+1+i}\left(3-|\mathcal{N}(v_j)\cap V|\right)$: Counts the number of combinations of collapse choices for all \SPs with a neighboring terminal that have already been yet forced to collapse with a terminal, and now are forced to merge with a neighboring \SP. Each of them can merge with as many \SPs neighbors as they have.
\end{itemize}
