# Supplementary material for: The Central Spanning Tree Problem
Source: arXiv:2404.06447 source file (2024-04-09)
Supplement: Supplementary file 4 [file GRASP_PR_comparison.tex]

In this section, we delve into assessing our heuristic's performance on large instances. Utilizing the GRASP\_PR algorithm, we compute the \CST across various $\alpha$ values, comparing the results with our \mSTreg heuristic on the OR library datasets. Before proceeding, we will briefly outline the GRASP\_PR algorithm proposed by \cite{sattari_metaheuristic_2015}.

\subsection{GRASP\_PR by \cite{sattari_metaheuristic_2015}}
GRASP\_PR (Greedy Randomized Adaptive Search Procedure with Path Relinking) is a metaheuristic for combinatorial optimization. \cite{sattari_metaheuristic_2015}, adapted the general purpose GRASP\_PR to solve the MRCT. The algorithm comprises three phases:

\begin{itemize}[leftmargin=*]
	\item Construction Phase (Greedy): Acknowledging that the shortest path tree with minimum cost offers a 2-approximation of the optimal MRCT, the authors designate roots as nodes whose shortest path trees incur lower costs. A random tree is then built by initially selecting a root at random. Following a process akin to Prim's algorithm, vertices are added to the tree by sampling edges, prioritizing shorter edges for higher selection probability.
	
	\item Local search: This phase iteratively refines the solution by swapping pairs of edges. Specifically, each iteration targets the pair of edges (one inside and one outside the tree) that most effectively reduces the overall cost. This iterative process continues until it converges to a local minimum, i.e. no further reduction in cost is achievable. Note that each iteration of the local search attempts to swap all pairs of valid edges to identify the one that achieves the maximum reduction in cost. Consequently, in a complete graph, the complexity of each iteration is $\mathcal{O}(n^2)$, where $n$ represents the number of nodes.
	
	\item Path Relinking Phase: Explores paths between high-quality solutions by swapping edges between good quality trees until one transforms into the other. The complexity of this step depends on the number of edges that the trees share in common.
\end{itemize}

\subsection{Comparison of GRASP\_PR with mSTreg for the general $\operatorname{CST}$}
The previous section provided an overview of the GRASP\_PR algorithm by \cite{sattari_metaheuristic_2015}. It's important to note that the overall complexity is dominated by the local search, scaling quadratically with the number of nodes. In contrast, the \mSTreg complexity per iteration is $\mathcal{O}(dn\log(n)^2)$ (Appendix K), rendering \mSTreg more efficient.

Additionally, GRASP\_PR requires an initial random guess to initiate the local search. The quality of this guess impacts the number of iterations needed for the local search to converge. We will show that initializing the local search with a solution generated by the \mSTreg allows for initializations that enhance the performance of GRASP\_PR. To ensure variability in the mSTreg output, we initialize it with random topologies instead of the \mST. Despite this modification, as the \mST initialization yielded favorable results, we opt to sample trees similar to it. To achieve this, we construct a tree by randomly sampling edges, prioritizing shorter ones. In concrete, we sample edge $(i,j)$ with probability proportional to $\exp(-||x_i-x_j||/T)$ for some temperature $T$. This sampling approach is akin to the one used in Karger's algorithm for approximating the minimum cut \citep{karger1993global,jenner2021extensions} and differs from the GRASP\_PR construction phase in that it doesn't require that one end of the edges belongs to the current tree.

While our main paper relied on GRASP\_PR MRCT costs from \cite{sattari_metaheuristic_2015}, we now validate our claims using our implementation of GRASP\_PR. Given that the GRASP\_PR is a versatile algorithm, we used it to compute the \CST with alternative $\alpha$ values besides 1.  Acknowledging that for lower $\alpha$ values, the optimum trees will be more similar to the \mST, we adapted the construction phase of GRASP\_PR. Specifically, for $\alpha<0.7$, it generates the random tree based on the Karger's sampling method mentioned above. For $\alpha\geq 0.7$, it uses the construction proposed by \cite{sattari_metaheuristic_2015}. Due to the relatively slow performance of our Python implementation of GRASP\_PR, we imposed a 5-minute time threshold. If exceeded, the algorithm returns the best solution at the end of the path relinking phase.

To assess performance, we conducted tests using GRASP\_PR, GRASP\_PR initialized with mSTreg (GRASP\_PR\_\mSTreg), and the mSTreg algorithms on OR library datasets for problems with 50 and 100 terminals. Analogously to the plots shown in the main paper, \figurename \ref{fig:GRASPPR_CST} displays the relative errors using GRASP\_PR\_\mSTreg cost as a reference for different $\alpha$ values in the set $\{0.2, 0.4, 0.6, 0.8, 1\}$. Notably, the combination of the mSTreg heuristic with GRASP\_PR consistently achieved the lowest cost, as all relative costs are above $0$, proving that the mSTreg can enhance GRASP\_PR performance.

Across 30 runs (combining 5 $\alpha$ values, 2 problem sizes, and 3 instances), GRASP\_PR outperformed mSTreg in only 12 instances. Moreover, achieving a lower cost took minutes for GRASP\_PR, while mSTreg run in the order of seconds. Consequently, mSTreg emerges as a favorable alternative, delivering a descent solution quickly.

\input{Figures/Appendix/GRASPR_CST.tex}
